# Supplementary material for: Prompt-Guided Environmentally Consistent Adversarial Patch
Source: arXiv:2411.10498 source file (2024-11-15)
Supplement: Supplementary file 1 [file X_suppl.tex]

\clearpage
\setcounter{page}{1}
\maketitlesupplementary

\section{More Experiments and Details}
\label{sec:more_experiments}

\subsection{Epoch Selection}
To strike a balance between overfitting and underfitting in the white-box models, selecting the right number of epochs is crucial. To this end, we conduct an experiment under the same settings as described in Section 4.1, using YOLOv5 as our white-box model.

As shown in Fig.~\ref{pics:total_loss}, the total loss stabilizes around 100 epochs. After this point, the loss does not decrease notably, indicating that further training would not lead to significant improvements. Continuing beyond this could result in overfitting, where the patch becomes overly specialized to the white-box model and performs poorly on unseen models. Therefore, we select 100 epochs as the final point for optimization.

\subsection{Influence of Diffusion Steps}
As is well-known, the number of diffusion steps plays a crucial role in determining the quality of generated images. In the DDIM setting, increasing the number of steps generally improves image quality, though it also raises computational costs. To explore the effect of diffusion steps on adversarial patches, we conduct an experiment by gradually increasing the number of steps from 4 to 9. Using YOLOv5 as our white-box model and following the experimental setup in Section 4.1, we present the generated patches in Fig.~\ref{fig:diffusion steps}.

As shown in the figure, with fewer diffusion steps, the generated patch aligns less with the text description \( \mathcal{P} \). However, as the number of steps increases, the patch progressively aligns more closely with the text. This suggests that, even in an adversarial setting, increasing diffusion steps strengthens the influence of the text on patch generation. To balance patch quality with computational efficiency, we set the number of diffusion steps to 7.

\begin{figure}[t]
  \centering
  \includegraphics[width=1.0\columnwidth]{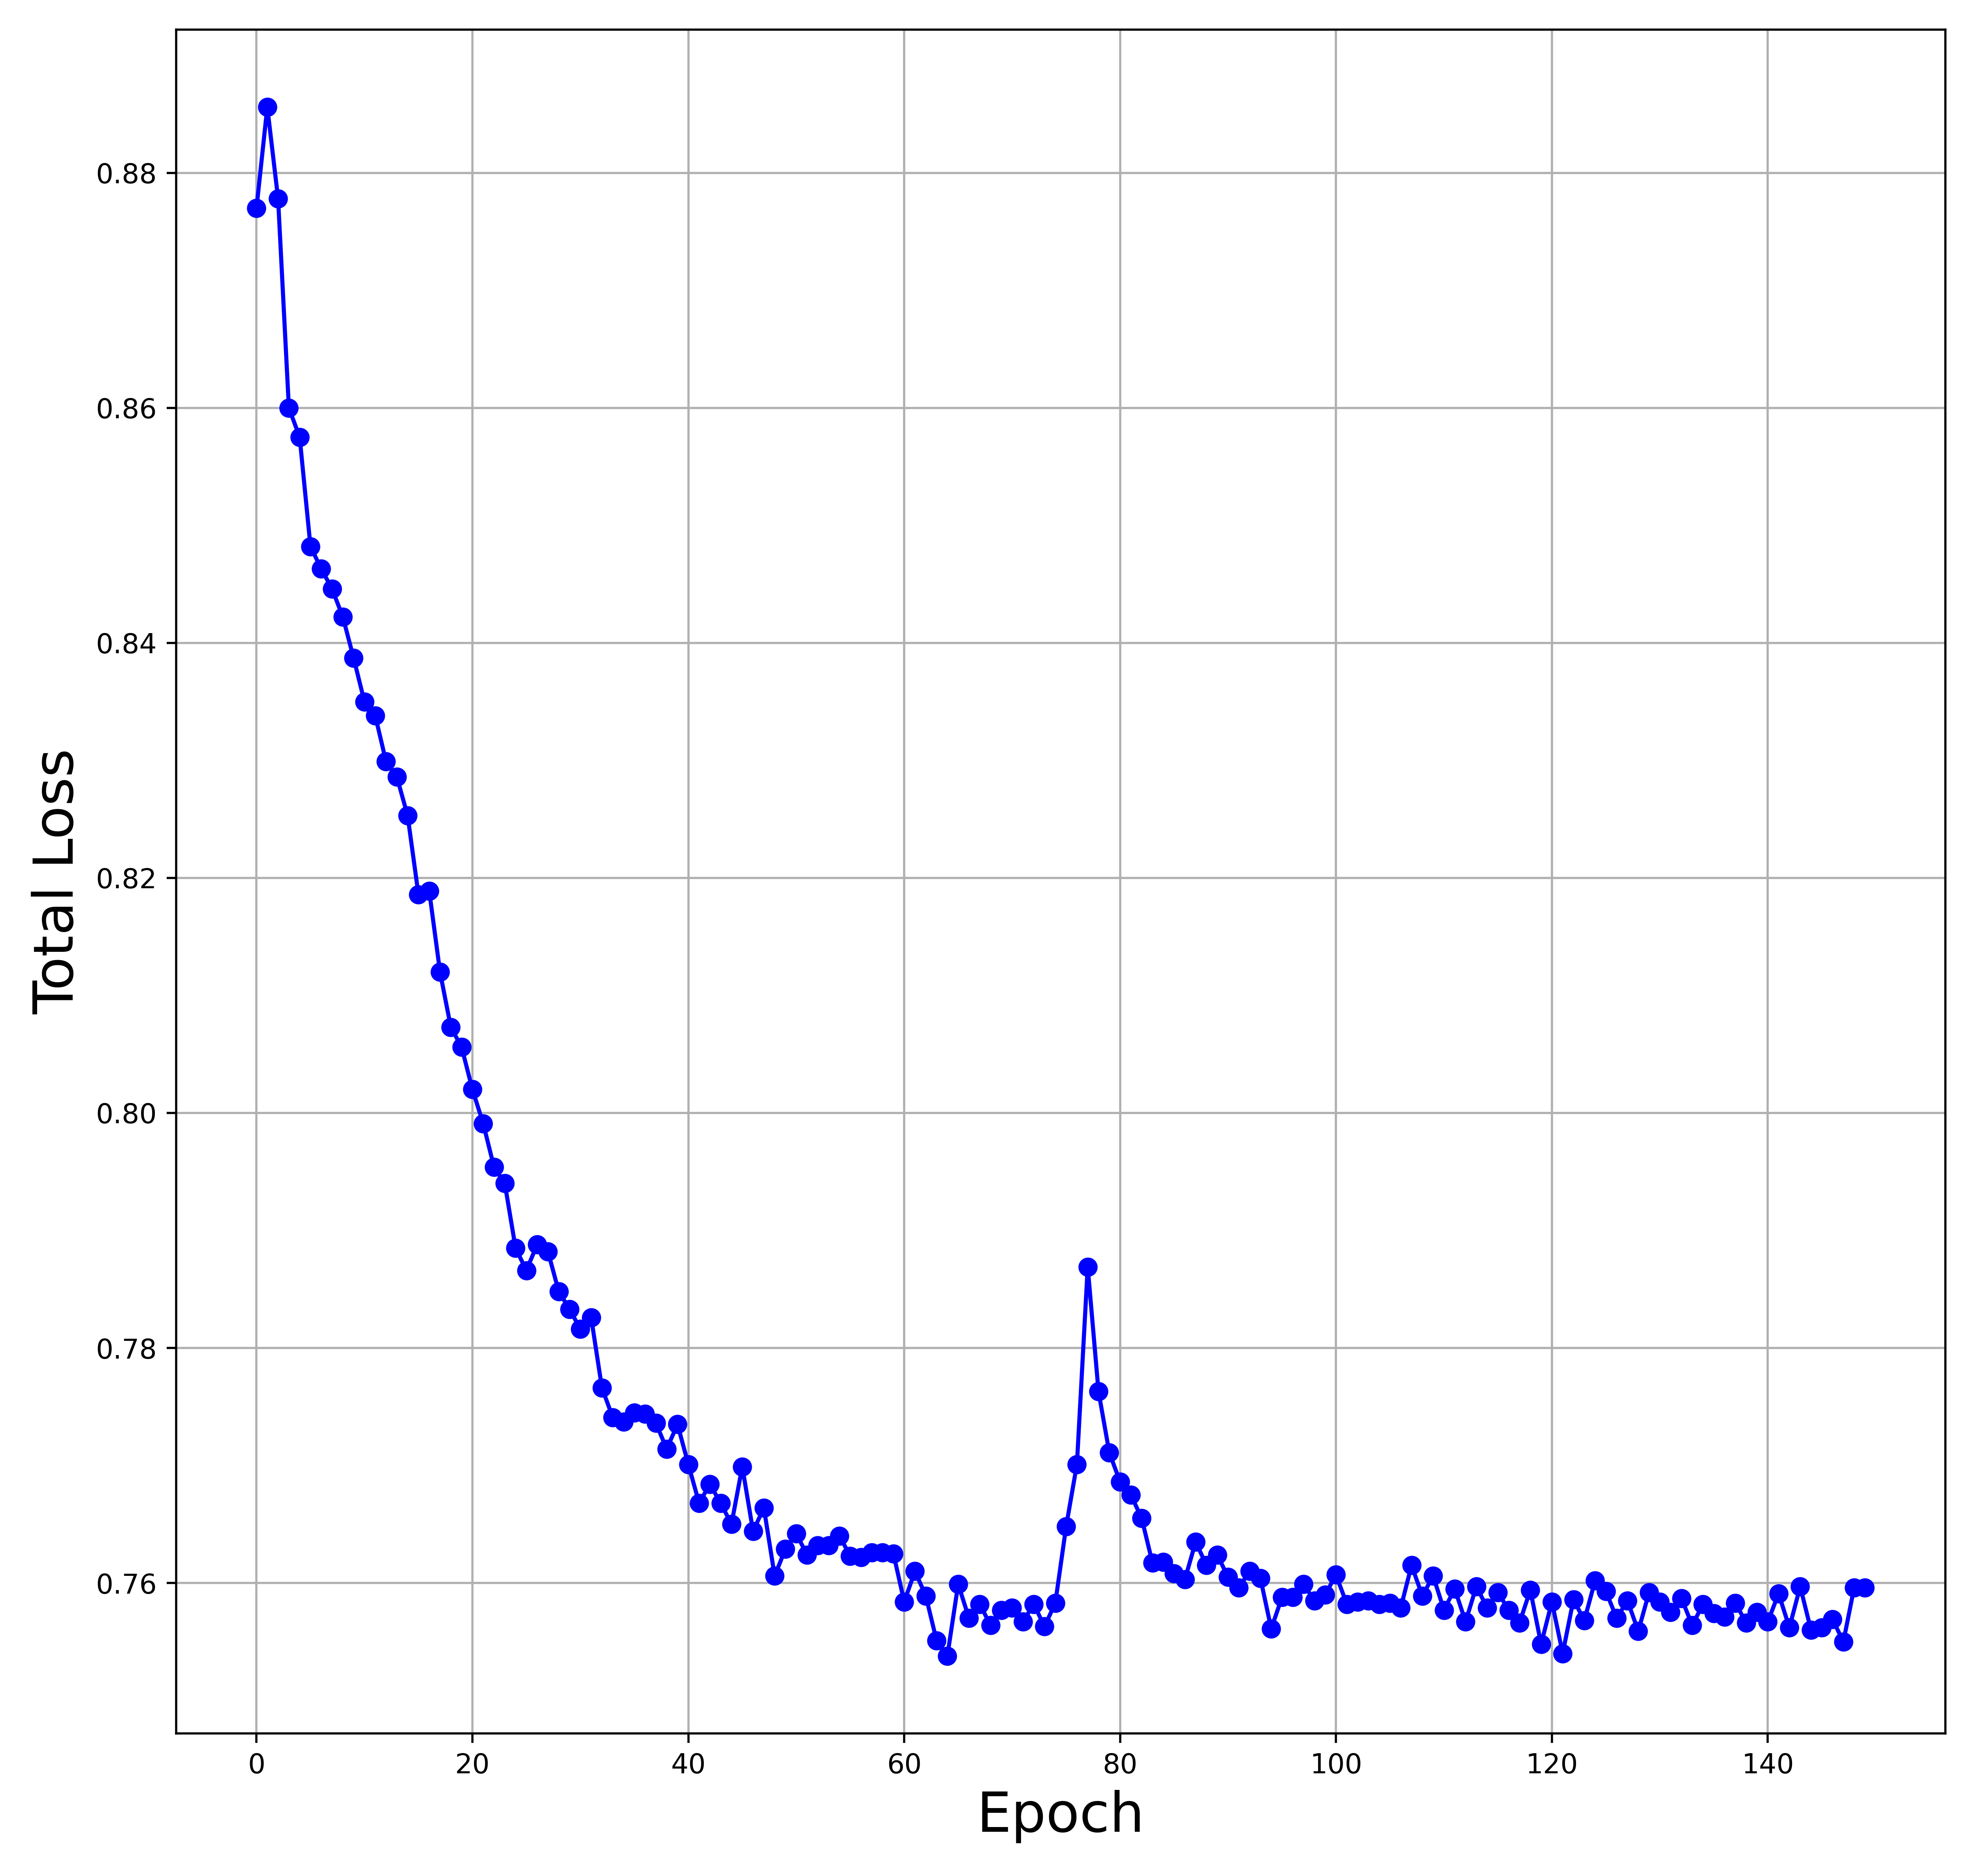}
  \caption{The total loss of PG-ECAP with respect to the epoch against the Yolov5.}
  \label{pics:total_loss}
\end{figure}

\begin{figure}[t]
  \centering
  \includegraphics[width=1.0\columnwidth]{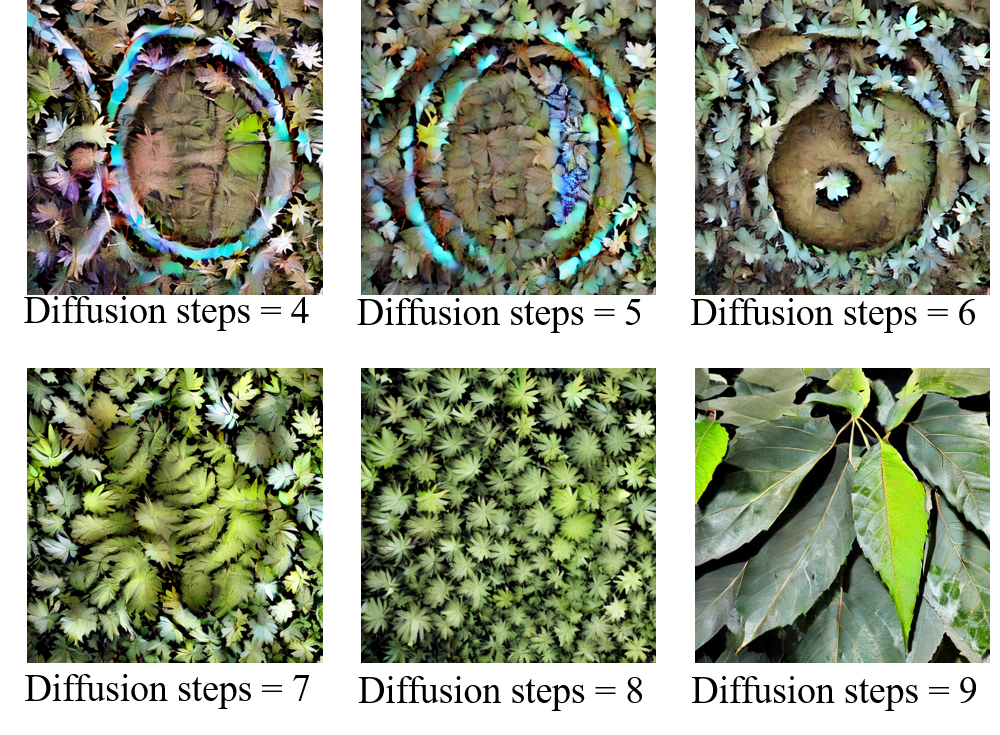}
  \caption{The generated patch under different diffusion steps, all these patches are generated by attacking Yolov5.}
  \label{fig:diffusion steps}
\end{figure}

\subsection{Influence of Patch Size}
To investigate the impact of patch size on the performance of our method, we conduct an ablation study across various patch scales: [0.32, 0.34, 0.36, 0.38, 0.40].

As shown in Fig.~\ref{pics:patch_size}, the $mAP_{50}$ decreases as the patch size increases. This trend suggests that larger patches are more effective in maintaining the performance of our method. Larger patches cover a greater area of the target object, making it more difficult for object detectors to identify the person. These results highlight that patch size is a critical factor in designing effective adversarial patches for object detection. They also illustrate the trade-off between patch size and performance: while larger patches are more effective, excessively large patches may not be practical for real-world applications. Therefore, selecting an optimal patch size is crucial for striking a balance between effectiveness and practicality.

\subsection{Physical Detection Results with More Postures and Conditions}
To further validate the effectiveness of our proposed method, we conduct additional experiments with our adversarial clothing under various postures and conditions. Specifically, we have two participants wear the clothing in turn and evaluate its performance across three additional postures—walking, spinning, and leaning—in two different indoor environments: a lobby and a hallway. 

Additionally, we account for potential occlusions of the adversarial clothing, as such occurrences are common in real-world settings. We test our clothing under two types of occlusion: single-hand occlusion, where part of the clothing is covered by one hand, and double-hand occlusion, where both hands cover the clothing. These tests simulate realistic conditions where the clothing may be partially obscured by the wearer’s hands.

The physical detection results are presented in Fig.~\ref{fig:physical_sup}. From the figure, it is clear that our clothing consistently enables participants to evade detection across all tested scenarios. This demonstrates the robustness of our method and its effectiveness in a wide range of real-world situations.

In summary, our additional tests, conducted under various postures, and occlusion conditions, show that our patch-based clothing is not only effective but also robust. These findings emphasize the practical value of our approach and its potential for real-world applications.

\begin{figure}[t]
  \centering
  \includegraphics[width=1.0\columnwidth]{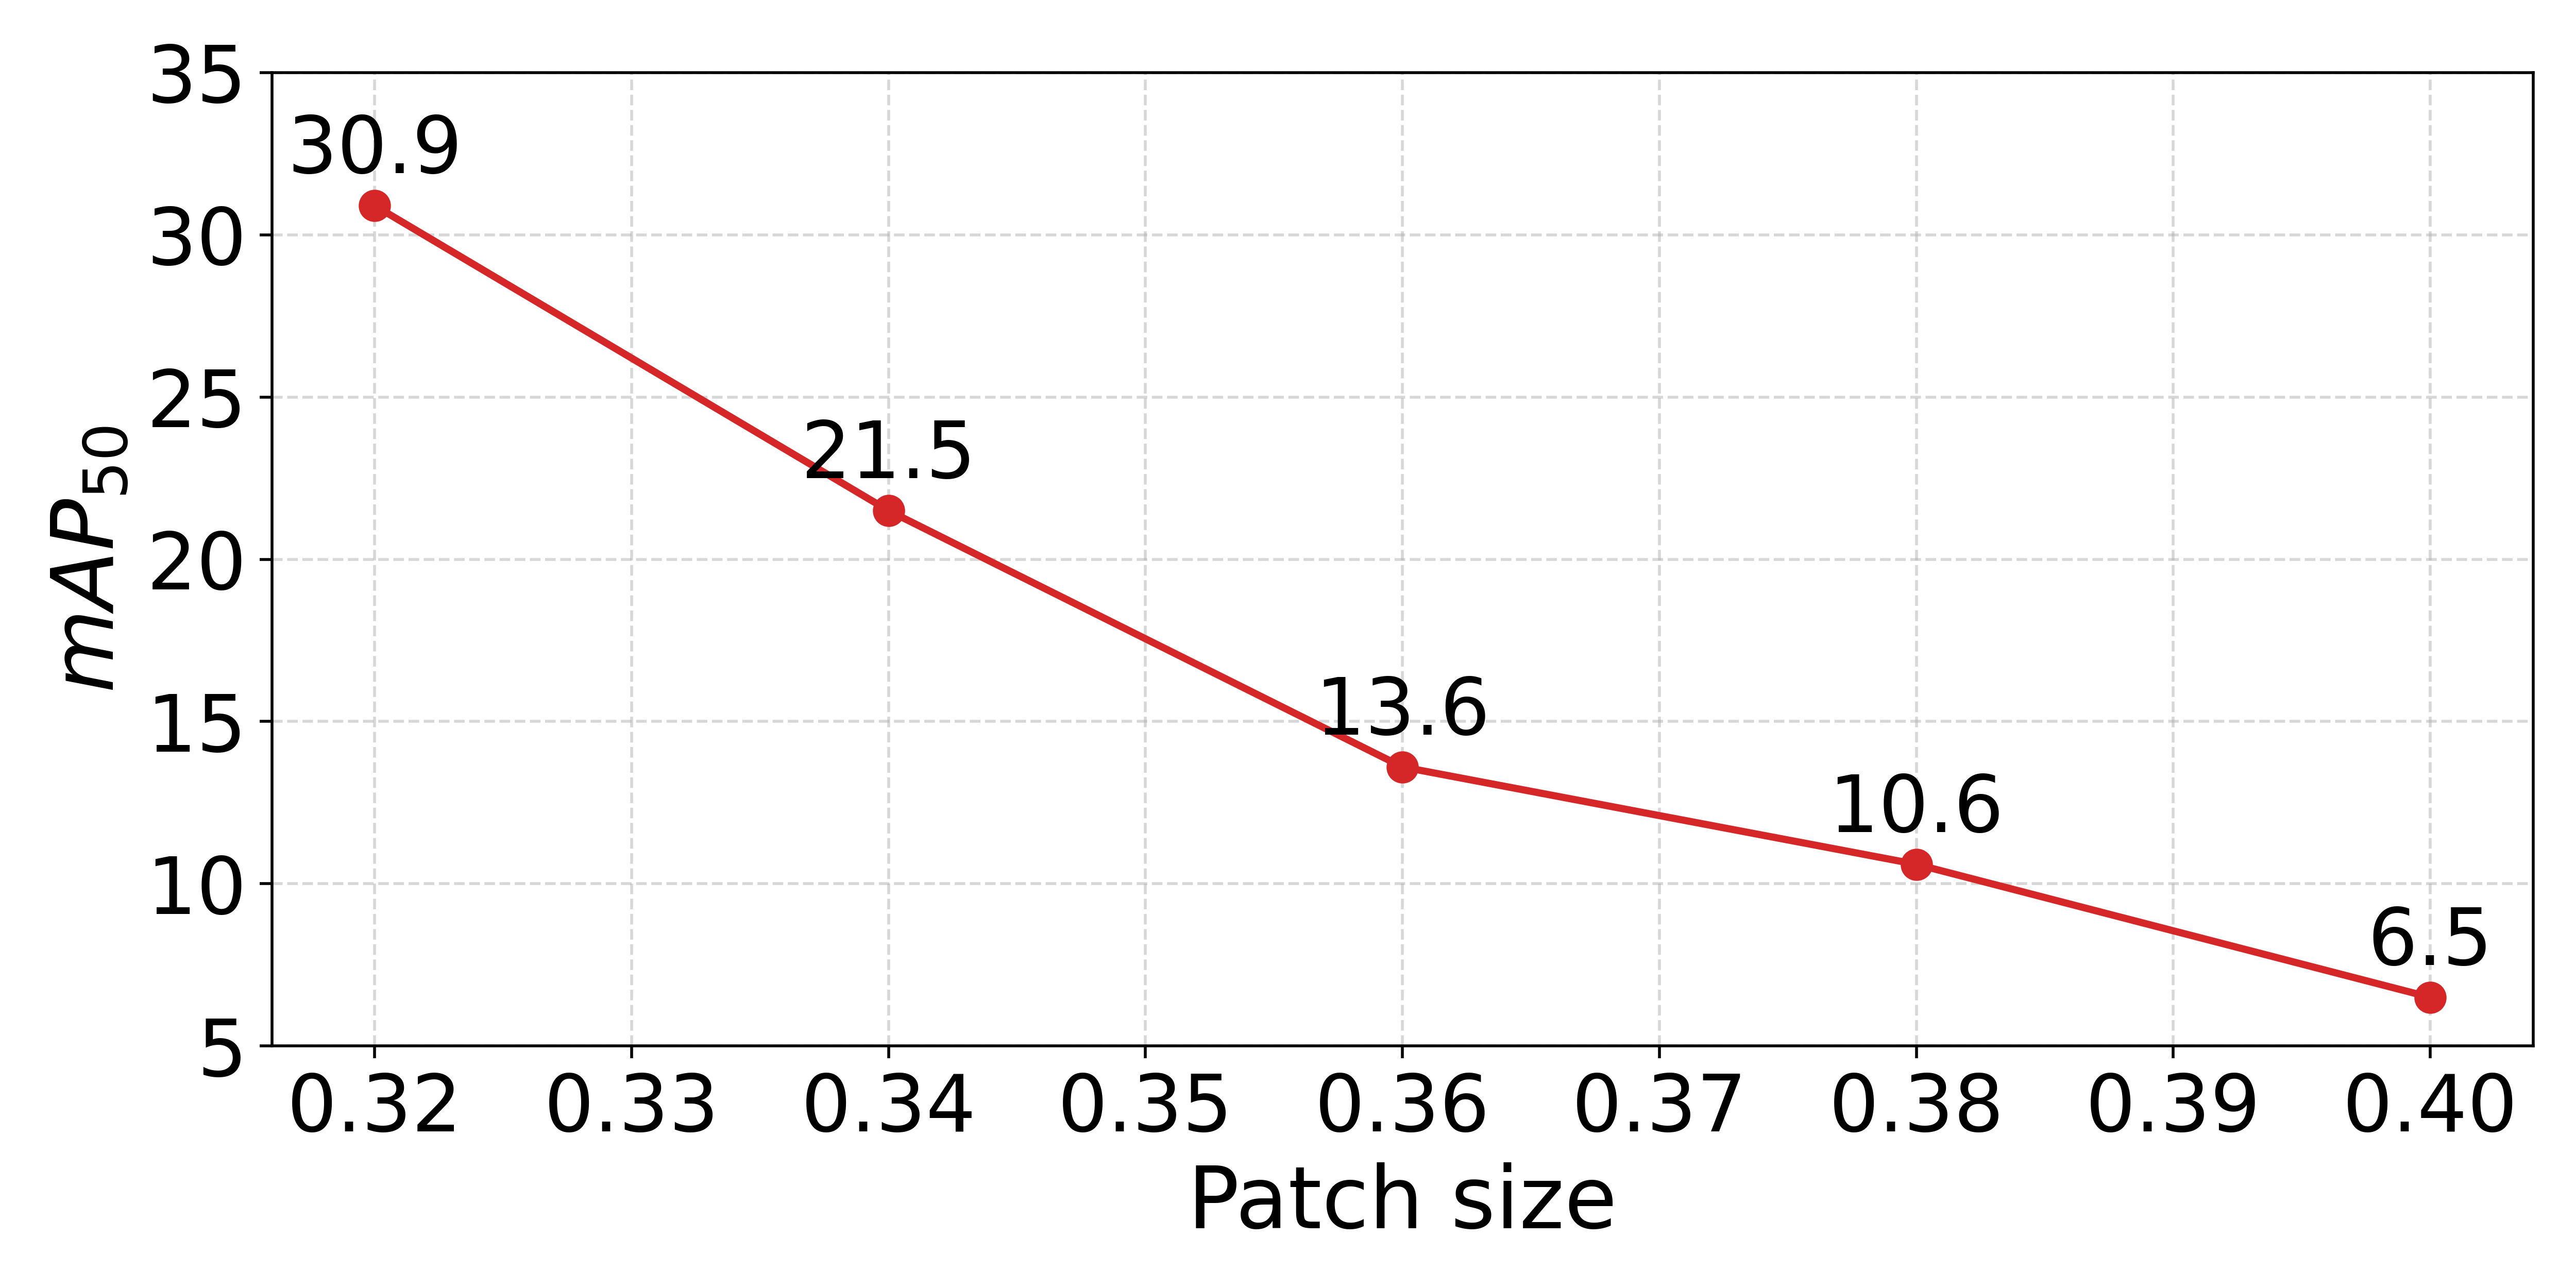}
  \caption{The results of adversarial patches with increasing patch size. All these adversarial patches are generated on Yolov5.}
  \label{pics:patch_size}
\end{figure}

\begin{table}[h]
    \centering
    \begin{adjustbox}{max width=\columnwidth}
    \begin{tabular}{>{\centering\arraybackslash}m{2.5cm}>{\centering\arraybackslash}m{1.5cm}>{\centering\arraybackslash}m{3cm}>{\centering\arraybackslash}m{3cm}}
        \toprule
        \multicolumn{1}{c}{\textbf{Transformations}} & \multicolumn{1}{c}{\textbf{Parameters}} & \multicolumn{1}{c}{\textbf{Description}} & \multicolumn{1}{c}{\textbf{Effect on Robustness}} \\
        \midrule
        Contrast & $[0.8, 1.2]$ & Adjusts the contrast of the image. & Improves robustness against variations in lighting conditions. \\
        \midrule
        Brightness & $\pm 0.1$ & Adjusts the brightness of the image. & Enhances robustness against changes in illumination. \\
        \midrule
        Noise & $\pm 0.1$ & Adds random noise to the image. & Increases robustness against sensor noise and image compression artifacts. \\
        \midrule
        Rotate & $\pm 20^\circ$ & Rotates the image within a specified range. & Improves robustness against slight rotations of the input image. \\
        \midrule
        Location & $\pm 0.1$ & Translates the image slightly. & Enhances robustness against minor shifts in the position of the object in the image. \\
        \bottomrule
    \end{tabular}
    \end{adjustbox}
    \caption{Transformations used in Expectation Over Transformation (EOT).}
    \label{tab:eot}
\end{table}

\subsection{Expectation Over Transformation (EOT)}
In this section, we detail the transformations employed in Expectation Over Transformation (EOT). EOT is a technique that enhances the robustness of adversarial attacks by considering multiple transformations. By applying a range of transformations, the attack becomes more robust to variations in real-world scenarios, thereby improving its effectiveness in practical applications.

The transformations used in EOT include adjustments to contrast, brightness, noise, rotation, and location. Each transformation is applied with specific parameters to simulate different real-world conditions. For instance, adjusting contrast and brightness simulates changes in lighting, while adding noise simulates sensor noise or image compression influence. Rotating the patch and changing its position can simulate slight movements and shifts of the patch on the object. 

The specific transformations, their parameters, descriptions, and their effects on robustness are listed in Tab.~\ref{tab:eot}. By incorporating these transformations, we ensure that our adversarial patches maintain their effectiveness across a wide range of conditions, thereby enhancing their practical utility.

\section{Limitations and Future Work}
\label{sec:Future work}
It is important to note that, in this study, we simply attach the generated patch to the T-shirt, which limits the attack’s effectiveness in the physical world. To overcome this limitation, future work could explore integrating diffusion models with 3D rendering techniques. By rendering the patch across the entire surface of the object, the attack’s robustness could be enhanced, making it more applicable in practical situations.

\begin{figure*}[t]
  \centering
  \includegraphics[width=\textwidth]{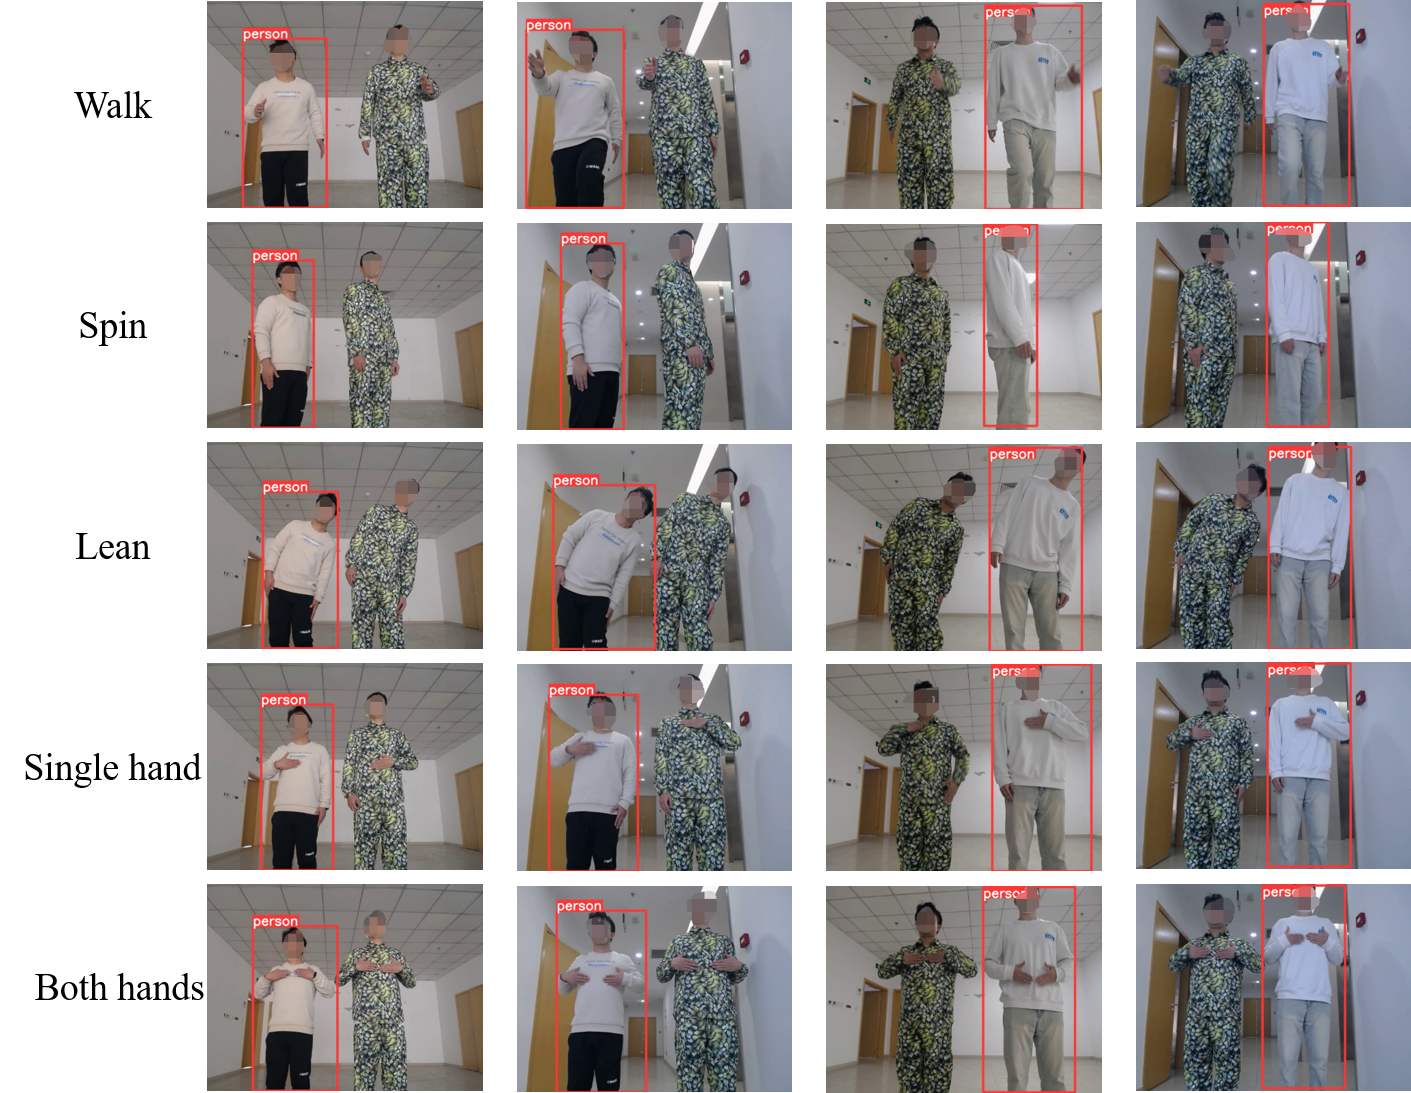}
  \caption{Detection results for three additional postures—walking, spinning, and leaning—and two types of occlusion: single-hand and both-hands.}
  \label{fig:physical_sup}
\end{figure*}
